# Supplementary material for: Evaluation of Orientation Ambiguity and Detection Rate in April Tag and WhyCode
Source: arXiv:2203.10180 source file (2022-11-11)
Supplement: Supplementary file 1 [file auto_generated_appendix_figures.tex]

\section{Test Case: calibration-z0.96 }
\begin{figure}
\centering
\includegraphics[width=\linewidth]{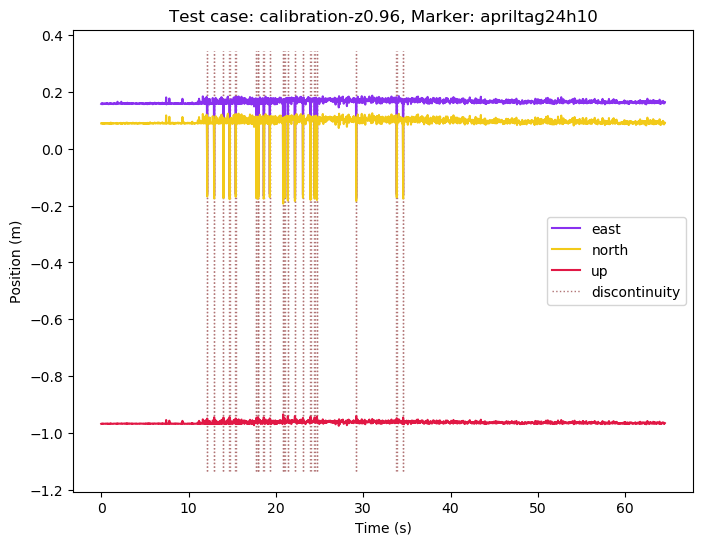}
\caption{ Test case: calibration-z0.96, Fiducial system: apriltag24h10 }
\end{figure}

\begin{figure}
\centering
\includegraphics[width=\linewidth]{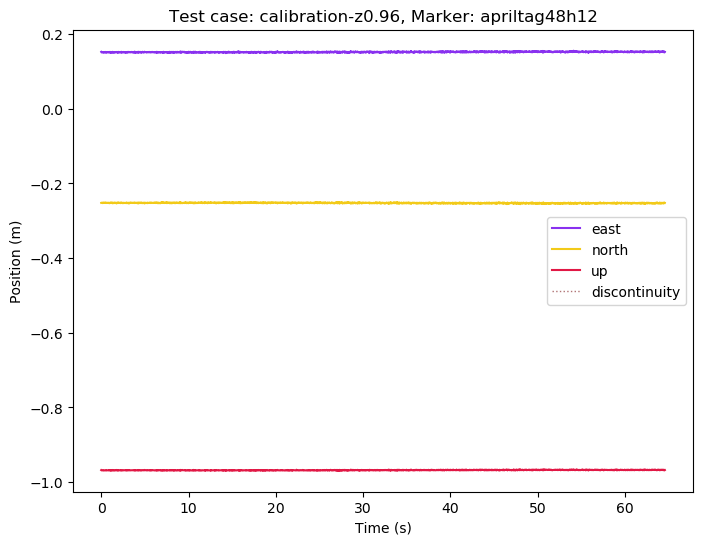}
\caption{ Test case: calibration-z0.96, Fiducial system: apriltag48h12 }
\end{figure}

\begin{figure}
\centering
\includegraphics[width=\linewidth]{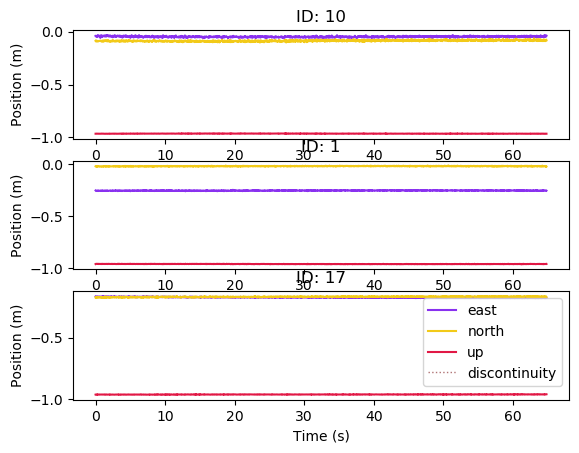}
\caption{ Test case: calibration-z0.96, Fiducial system: whycode-ellipse }
\end{figure}

\begin{figure}
\centering
\includegraphics[width=\linewidth]{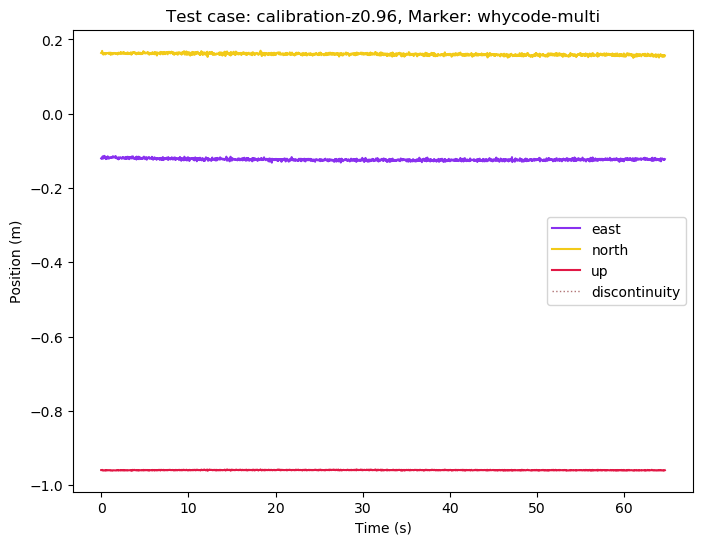}
\caption{ Test case: calibration-z0.96, Fiducial system: whycode-multi }
\end{figure}

\begin{figure}
\centering
\includegraphics[width=\linewidth]{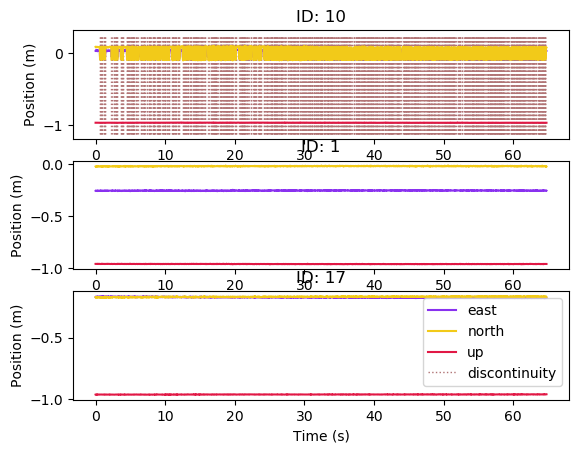}
\caption{ Test case: calibration-z0.96, Fiducial system: whycode-orig }
\end{figure}

\section{Test Case: east-west }
\begin{figure}
\centering
\includegraphics[width=\linewidth]{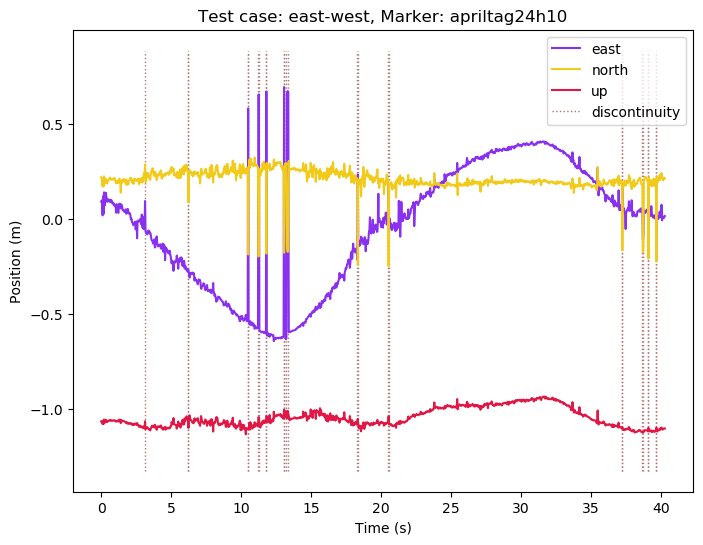}
\caption{ Test case: east-west, Fiducial system: apriltag24h10 }
\end{figure}

\begin{figure}
\centering
\includegraphics[width=\linewidth]{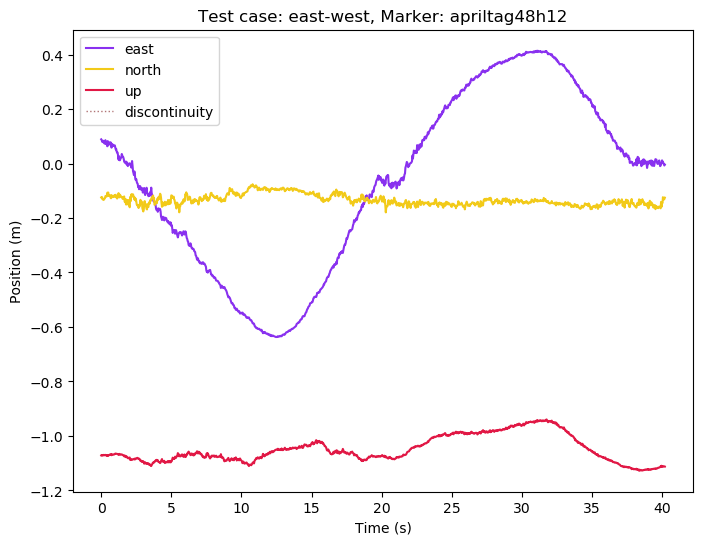}
\caption{ Test case: east-west, Fiducial system: apriltag48h12 }
\end{figure}

\begin{figure}
\centering
\includegraphics[width=\linewidth]{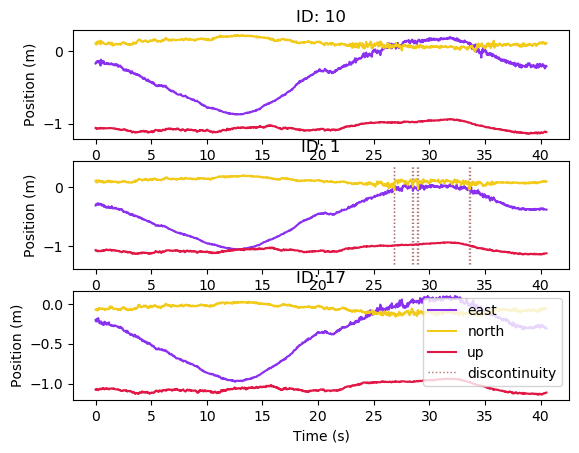}
\caption{ Test case: east-west, Fiducial system: whycode-ellipse }
\end{figure}

\begin{figure}
\centering
\includegraphics[width=\linewidth]{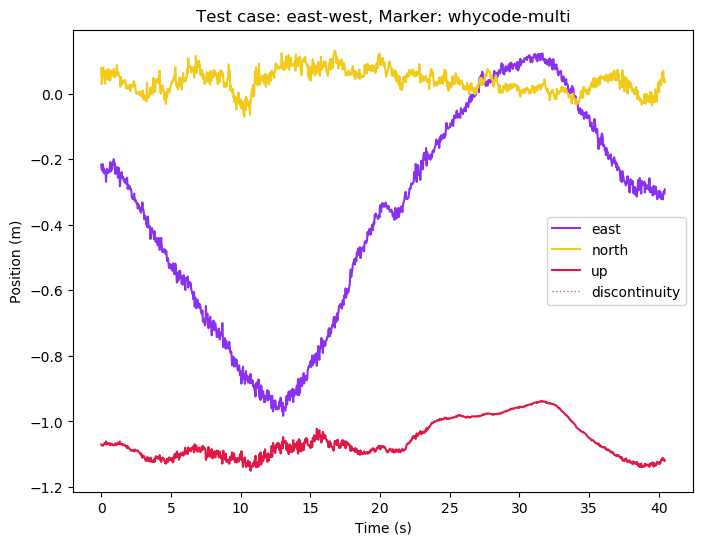}
\caption{ Test case: east-west, Fiducial system: whycode-multi }
\end{figure}

\begin{figure}
\centering
\includegraphics[width=\linewidth]{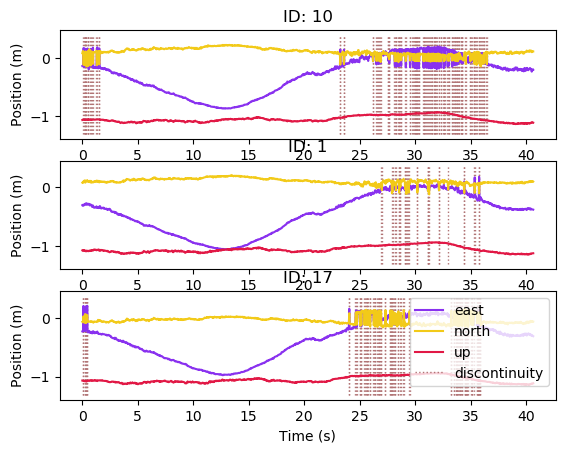}
\caption{ Test case: east-west, Fiducial system: whycode-orig }
\end{figure}

\section{Test Case: in-out-1 }
\begin{figure}
\centering
\includegraphics[width=\linewidth]{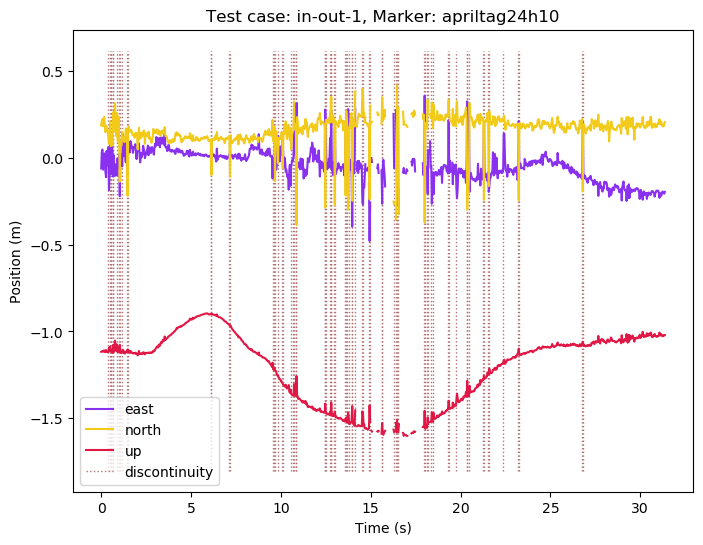}
\caption{ Test case: in-out-1, Fiducial system: apriltag24h10 }
\end{figure}

\begin{figure}
\centering
\includegraphics[width=\linewidth]{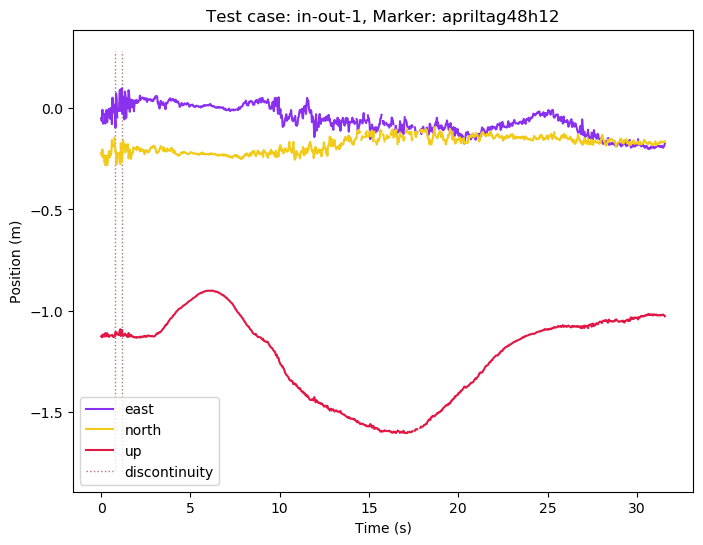}
\caption{ Test case: in-out-1, Fiducial system: apriltag48h12 }
\end{figure}

\begin{figure}
\centering
\includegraphics[width=\linewidth]{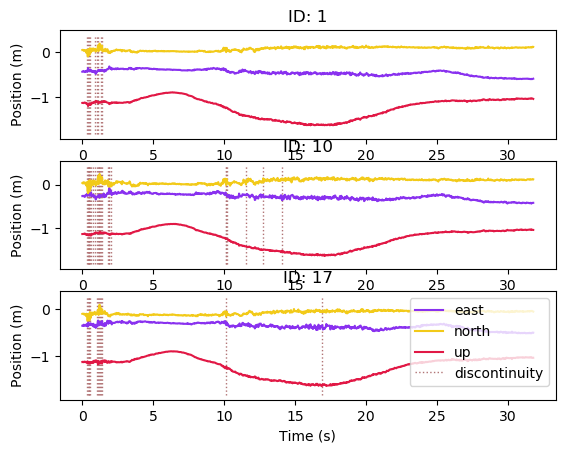}
\caption{ Test case: in-out-1, Fiducial system: whycode-ellipse }
\end{figure}

\begin{figure}
\centering
\includegraphics[width=\linewidth]{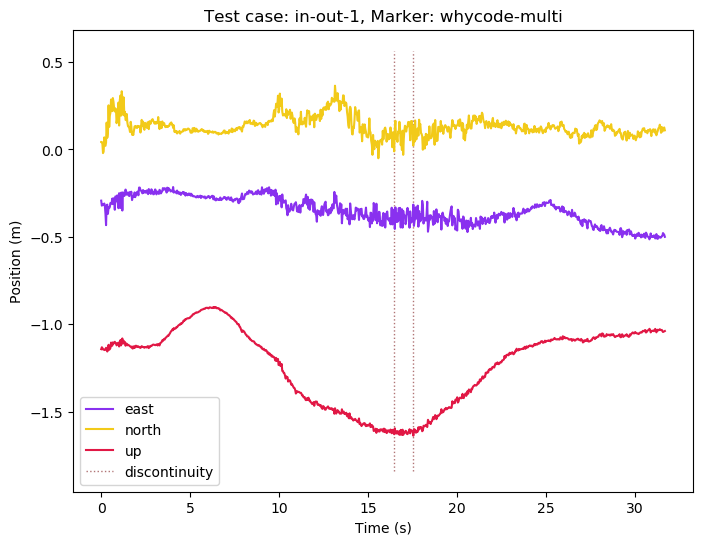}
\caption{ Test case: in-out-1, Fiducial system: whycode-multi }
\end{figure}

\begin{figure}
\centering
\includegraphics[width=\linewidth]{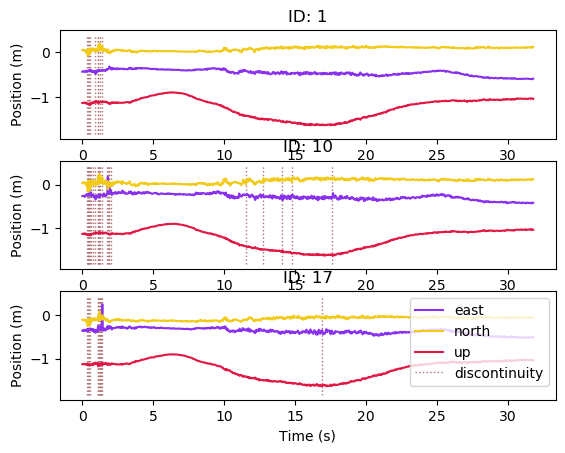}
\caption{ Test case: in-out-1, Fiducial system: whycode-orig }
\end{figure}

\section{Test Case: in-out-2 }
\begin{figure}
\centering
\includegraphics[width=\linewidth]{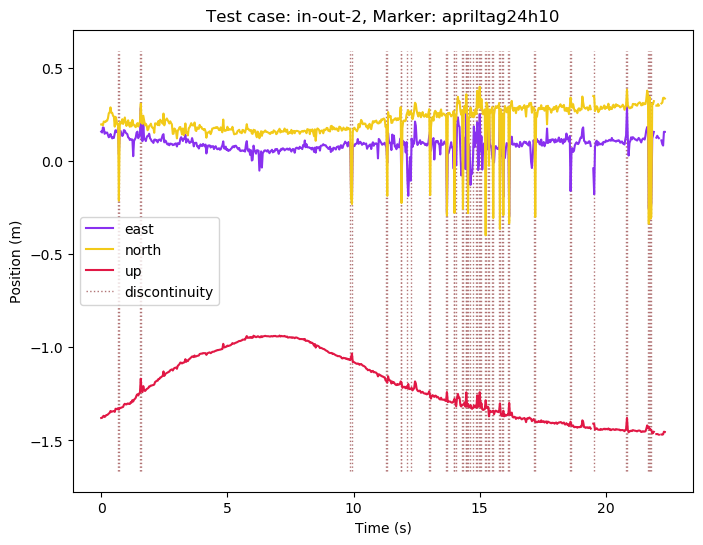}
\caption{ Test case: in-out-2, Fiducial system: apriltag24h10 }
\end{figure}

\begin{figure}
\centering
\includegraphics[width=\linewidth]{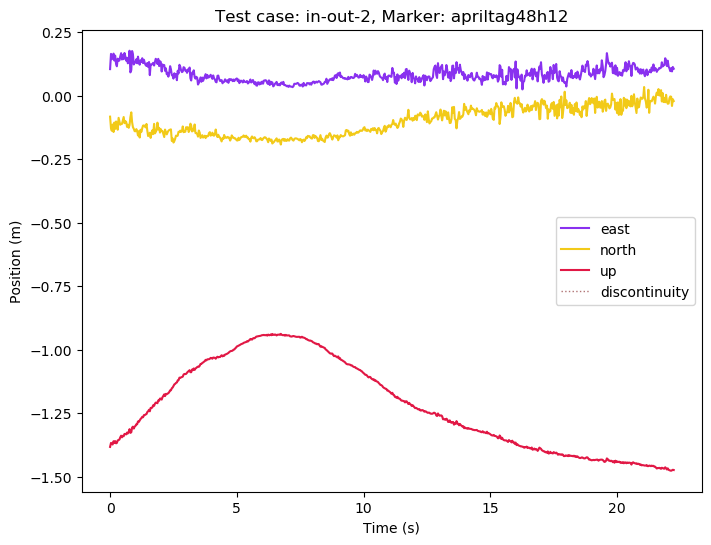}
\caption{ Test case: in-out-2, Fiducial system: apriltag48h12 }
\end{figure}

\begin{figure}
\centering
\includegraphics[width=\linewidth]{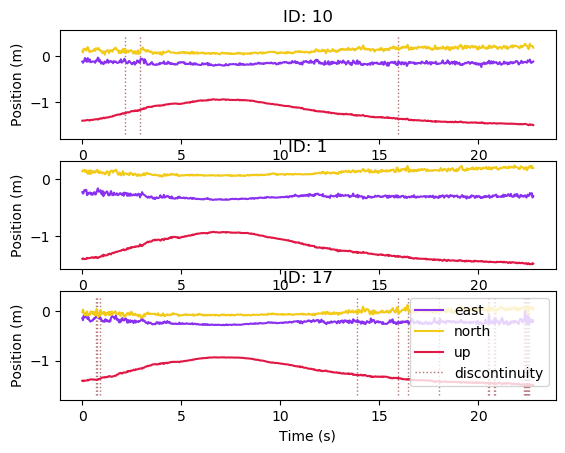}
\caption{ Test case: in-out-2, Fiducial system: whycode-ellipse }
\end{figure}

\begin{figure}
\centering
\includegraphics[width=\linewidth]{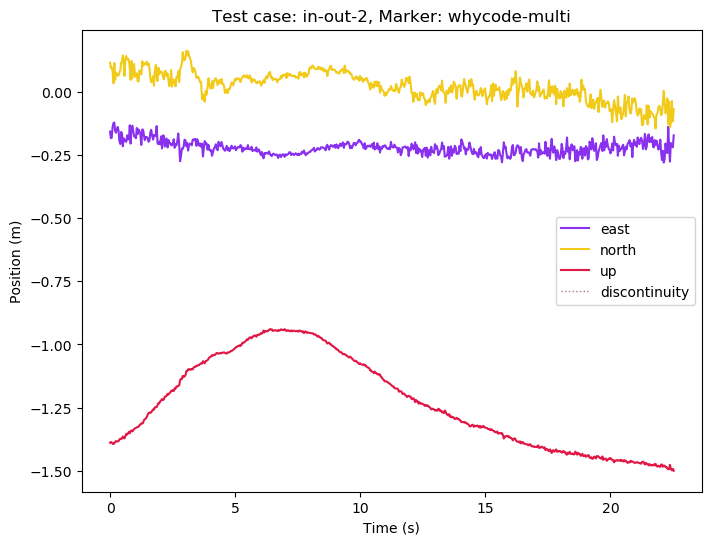}
\caption{ Test case: in-out-2, Fiducial system: whycode-multi }
\end{figure}

\begin{figure}
\centering
\includegraphics[width=\linewidth]{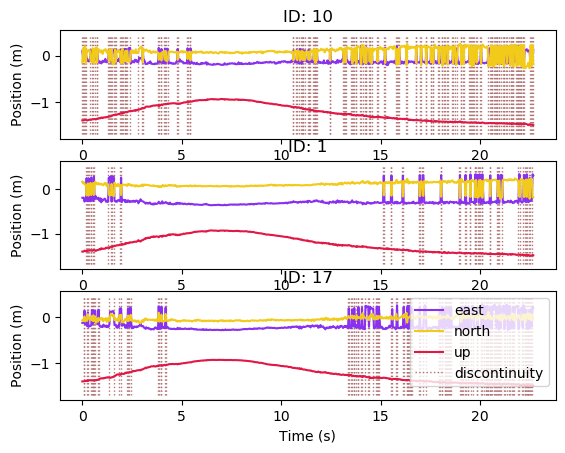}
\caption{ Test case: in-out-2, Fiducial system: whycode-orig }
\end{figure}

\section{Test Case: north-south }
\begin{figure}
\centering
\includegraphics[width=\linewidth]{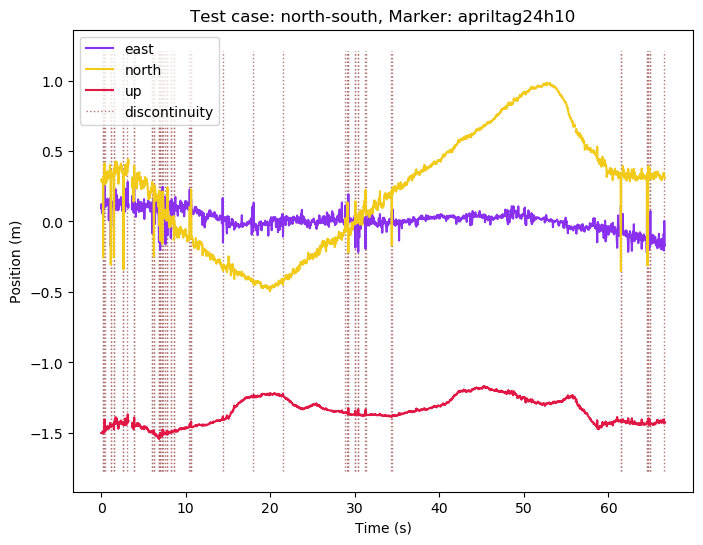}
\caption{ Test case: north-south, Fiducial system: apriltag24h10 }
\end{figure}

\begin{figure}
\centering
\includegraphics[width=\linewidth]{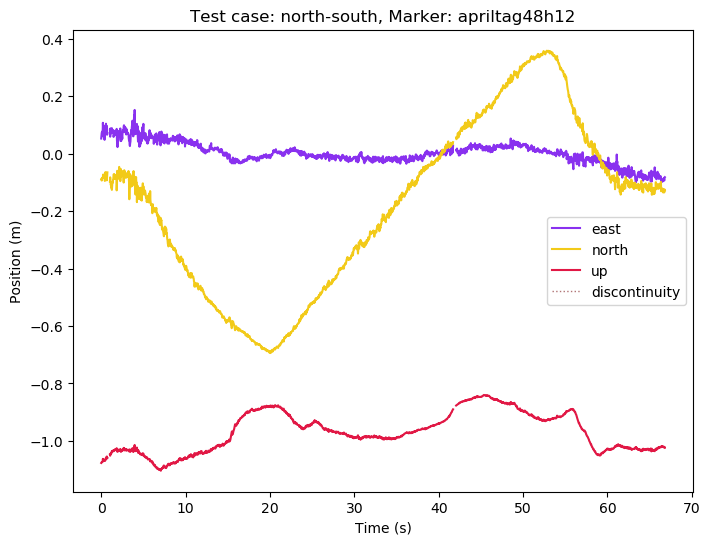}
\caption{ Test case: north-south, Fiducial system: apriltag48h12 }
\end{figure}

\begin{figure}
\centering
\includegraphics[width=\linewidth]{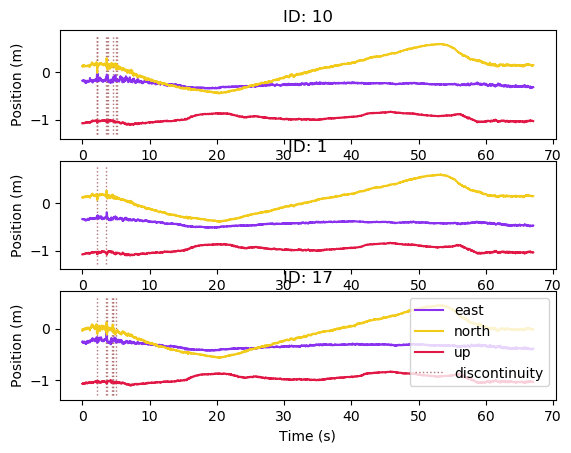}
\caption{ Test case: north-south, Fiducial system: whycode-ellipse }
\end{figure}

\begin{figure}
\centering
\includegraphics[width=\linewidth]{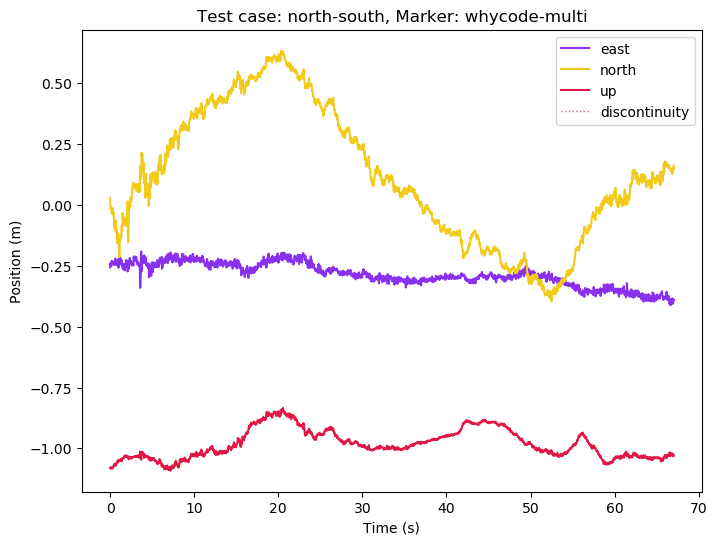}
\caption{ Test case: north-south, Fiducial system: whycode-multi }
\end{figure}

\begin{figure}
\centering
\includegraphics[width=\linewidth]{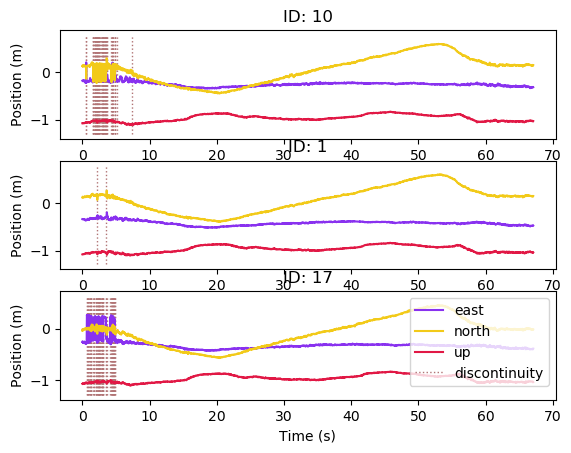}
\caption{ Test case: north-south, Fiducial system: whycode-orig }
\end{figure}
