# Supplementary material for: Evaluation of Orientation Ambiguity and Detection Rate in April Tag and WhyCode
Source: arXiv:2203.10180 source file (2022-11-11)
Supplement: Supplementary file 2 [file appendices.tex]

\subsection{Discontinuity Test Cases}
\label{appendix:discontinuity_test_cases}

Tables~\ref{table:single_marker_discontinuity_test_cases} and~\ref{table:bundle_discontinuity_test_cases} outline the
test cases for discontinuities in the single marker and bundle systems respectively.
Test cases with the same base name but different indices (e.g.~in-out-1 and in-out-2) are collected with the camera at
different distances from the fiducial marker(s), and the distance increases with the index.
These are not repeated measures.

\begin{table}[h]
    \centering
    \begin{tabular}{|lrr|rrr|rrr|rrr|rrr|}
\toprule
         Test Case & Length (s) & Frames & \multicolumn{3}{c|}{April Tag 24h10} & \multicolumn{3}{c|}{April Tag 48h12} & \multicolumn{3}{c|}{WhyCode Ellipse} & \multicolumn{3}{c|}{WhyCode Orig} \\
                 &          &      &             $n$ & $d$ & $r_d$ &             $n$ & $d$ & $r_d$ &             $n$ & $d$ & $r_d$ &          $n$ & $d$ & $r_d$ \\
\midrule
 calibration-z1.42 &     30.769 &    924 &             924 &   0 & 0.000 &             924 &   0 & 0.000 &             922 &   0 & 0.000 &          918 &   0 & 0.000 \\
          in-out-1 &     20.862 &    627 &             627 &  91 & 0.145 &             627 &   0 & 0.000 &             624 &   1 & 0.002 &          627 &   1 & 0.002 \\
          in-out-2 &     17.630 &    530 &             530 & 161 & 0.304 &             530 &   1 & 0.002 &             524 &   0 & 0.000 &          530 &   0 & 0.000 \\
          in-out-3 &     20.697 &    622 &             622 & 167 & 0.268 &             622 &   2 & 0.003 &             620 &   0 & 0.000 &          620 &   0 & 0.000 \\
          in-out-4 &     24.062 &    723 &             723 & 340 & 0.470 &             723 &  54 & 0.075 &             721 &   0 & 0.000 &          719 &  63 & 0.088 \\
      left-right-1 &     28.330 &    851 &             851 &   7 & 0.008 &             851 &   0 & 0.000 &             848 &  12 & 0.014 &          850 & 148 & 0.174 \\
      left-right-2 &     24.865 &    747 &             747 &   1 & 0.001 &             747 &   1 & 0.001 &             746 &   0 & 0.000 &          744 &   0 & 0.000 \\
      left-right-3 &     22.731 &    683 &             683 &   0 & 0.000 &             683 &   0 & 0.000 &             681 &   0 & 0.000 &          679 &   0 & 0.000 \\
      left-right-4 &     20.499 &    616 &             616 & 290 & 0.471 &             616 &  51 & 0.083 &             615 &   3 & 0.005 &          615 &  72 & 0.117 \\
orbit-left-right-1 &     54.567 &   1638 &            1638 &  34 & 0.021 &            1638 &   0 & 0.000 &            1631 &   0 & 0.000 &         1635 &   0 & 0.000 \\
orbit-left-right-2 &     41.096 &   1234 &            1234 &   0 & 0.000 &            1234 &   0 & 0.000 &            1229 &   0 & 0.000 &         1229 &   0 & 0.000 \\
orbit-left-right-3 &     56.131 &   1685 &            1685 &  73 & 0.043 &            1685 &   0 & 0.000 &            1681 &   0 & 0.000 &         1682 &   0 & 0.000 \\
orbit-left-right-4 &     40.833 &   1226 &            1226 & 350 & 0.285 &            1226 &  33 & 0.027 &            1220 &  16 & 0.013 &         1225 &  84 & 0.069 \\
   orbit-up-down-1 &     91.032 &   2732 &            2732 &   7 & 0.003 &            2732 &   0 & 0.000 &            2709 &   0 & 0.000 &         2724 &   0 & 0.000 \\
   orbit-up-down-2 &     80.296 &   2410 &            2410 &   6 & 0.002 &            2410 &   2 & 0.001 &            2403 &   0 & 0.000 &         2402 &   0 & 0.000 \\
   orbit-up-down-3 &     55.998 &   1681 &            1681 &   0 & 0.000 &            1681 &   0 & 0.000 &            1645 &   0 & 0.000 &         1671 &   0 & 0.000 \\
   orbit-up-down-4 &     58.999 &   1771 &            1771 & 374 & 0.211 &            1771 & 135 & 0.076 &            1761 &  48 & 0.027 &         1760 & 188 & 0.107 \\
  pan-left-right-1 &     40.398 &   1213 &            1213 &  18 & 0.015 &            1213 &   4 & 0.003 &            1205 &   4 & 0.003 &         1207 & 109 & 0.090 \\
  pan-left-right-2 &     43.829 &   1316 &            1316 &  28 & 0.021 &            1316 &  18 & 0.014 &            1308 &   0 & 0.000 &         1311 &  79 & 0.060 \\
  pan-left-right-3 &     39.430 &   1184 &            1184 &  18 & 0.015 &            1184 &   8 & 0.007 &            1179 &   2 & 0.002 &         1183 &  64 & 0.054 \\
  pan-left-right-4 &     28.563 &    858 &             858 & 322 & 0.375 &             858 &  86 & 0.100 &             858 &  76 & 0.089 &          858 & 174 & 0.203 \\
      randomized-1 &     39.730 &   1193 &            1193 & 377 & 0.316 &            1193 &  30 & 0.025 &            1183 &   1 & 0.001 &         1186 &   0 & 0.000 \\
      randomized-2 &     24.365 &    732 &             732 & 257 & 0.351 &             732 &  16 & 0.022 &             725 &  20 & 0.028 &          726 &  24 & 0.033 \\
      randomized-3 &     31.199 &    937 &             937 & 382 & 0.408 &             937 &  51 & 0.054 &             930 &  50 & 0.054 &          929 &  73 & 0.079 \\
      randomized-4 &     36.799 &   1105 &            1105 & 460 & 0.416 &            1105 & 168 & 0.152 &            1094 & 109 & 0.100 &         1093 & 129 & 0.118 \\
    tilt-up-down-1 &     29.998 &    901 &             901 &   8 & 0.009 &             901 &   0 & 0.000 &             897 &   0 & 0.000 &          897 &   0 & 0.000 \\
    tilt-up-down-2 &     41.301 &   1240 &            1240 &  57 & 0.046 &            1240 &   0 & 0.000 &            1234 &   1 & 0.001 &         1237 &  93 & 0.075 \\
    tilt-up-down-3 &     29.632 &    890 &             890 &  53 & 0.060 &             890 &   4 & 0.004 &             886 &   0 & 0.000 &          886 &   0 & 0.000 \\
    tilt-up-down-4 &     37.931 &   1139 &            1139 & 367 & 0.322 &            1139 & 100 & 0.088 &            1134 &  81 & 0.071 &         1137 & 355 & 0.312 \\
         up-down-1 &     33.167 &    996 &             996 &  70 & 0.070 &             996 &  10 & 0.010 &             993 &   0 & 0.000 &          993 &   0 & 0.000 \\
         up-down-2 &     31.998 &    961 &             961 & 216 & 0.225 &             961 &  21 & 0.022 &             958 &   0 & 0.000 &          958 &   0 & 0.000 \\
         up-down-3 &     39.030 &   1172 &            1172 &  87 & 0.074 &            1172 &   0 & 0.000 &            1166 &   0 & 0.000 &         1168 &   0 & 0.000 \\
         up-down-4 &     33.298 &   1000 &            1000 & 247 & 0.247 &            1000 &  70 & 0.070 &             999 &  58 & 0.058 &          999 & 279 & 0.279 \\
\bottomrule
\end{tabular}

    \caption{The test cases for discontinuity rates of the single marker systems. $n$ is the number of detections, $d$ is the number of discontinuities, and $r_d=\frac{d}{n}$ is the discontinuity rate for each test case.}
    \label{table:single_marker_discontinuity_test_cases}
\end{table}

\begin{table}[h]
    \centering
    \begin{tabular}{|lrr|rrr|rrr|rrr|}
\toprule
         Test Case & Length (s) & Frames & \multicolumn{3}{c|}{April Tag 24h10} & \multicolumn{3}{c|}{April Tag 48h12} & \multicolumn{3}{c|}{WhyCode Multi} \\
                 &          &      &             $n$ & $d$ & $r_d$ &             $n$ & $d$ & $r_d$ &           $n$ & $d$ & $r_d$ \\
\midrule
 calibration-z1.42 &     30.769 &    924 &             924 &   0 & 0.000 &             924 &   0 & 0.000 &           807 &   0 & 0.000 \\
          in-out-1 &     20.862 &    627 &             627 &  89 & 0.142 &             627 &   0 & 0.000 &           552 &  20 & 0.036 \\
          in-out-2 &     17.630 &    530 &             530 & 154 & 0.291 &             530 &   1 & 0.002 &           465 &   0 & 0.000 \\
          in-out-3 &     20.697 &    622 &             622 & 181 & 0.291 &             622 &   2 & 0.003 &           542 &   1 & 0.002 \\
          in-out-4 &     24.062 &    723 &             723 & 341 & 0.472 &             723 &  54 & 0.075 &           641 & 146 & 0.228 \\
      left-right-1 &     28.330 &    851 &             851 &   6 & 0.007 &             851 &   0 & 0.000 &           748 &  30 & 0.040 \\
      left-right-2 &     24.865 &    747 &             747 &   2 & 0.003 &             747 &   0 & 0.000 &           652 &   1 & 0.002 \\
      left-right-3 &     22.731 &    683 &             683 &   0 & 0.000 &             683 &   0 & 0.000 &           597 &   0 & 0.000 \\
      left-right-4 &     20.499 &    616 &             616 & 290 & 0.471 &             616 &  51 & 0.083 &           553 & 138 & 0.250 \\
orbit-left-right-1 &     54.567 &   1638 &            1638 &  51 & 0.031 &            1638 &   0 & 0.000 &          1424 &   2 & 0.001 \\
orbit-left-right-2 &     41.096 &   1234 &            1234 & 107 & 0.087 &            1234 &   0 & 0.000 &          1074 &   2 & 0.002 \\
orbit-left-right-3 &     56.131 &   1685 &            1685 &  72 & 0.043 &            1685 &   0 & 0.000 &          1457 &   0 & 0.000 \\
orbit-left-right-4 &     40.833 &   1226 &            1226 & 350 & 0.285 &            1226 &  33 & 0.027 &          1079 & 109 & 0.101 \\
   orbit-up-down-1 &     91.032 &   2732 &            2732 &   3 & 0.001 &            2732 &   5 & 0.002 &          2396 &   0 & 0.000 \\
   orbit-up-down-2 &     80.296 &   2410 &            2410 &   5 & 0.002 &            2410 &   1 & 0.000 &          2089 &   0 & 0.000 \\
   orbit-up-down-3 &     55.998 &   1681 &            1681 &   0 & 0.000 &            1681 &   3 & 0.002 &          1469 &   0 & 0.000 \\
   orbit-up-down-4 &     58.999 &   1771 &            1771 & 374 & 0.211 &            1771 & 138 & 0.078 &          1557 & 300 & 0.193 \\
  pan-left-right-1 &     40.398 &   1213 &            1213 &  16 & 0.013 &            1213 &   2 & 0.002 &          1066 &  24 & 0.023 \\
  pan-left-right-2 &     43.829 &   1316 &            1316 &  27 & 0.021 &            1316 &  13 & 0.010 &          1156 &  19 & 0.016 \\
  pan-left-right-3 &     39.430 &   1184 &            1184 &  16 & 0.014 &            1184 &  10 & 0.008 &          1035 &  11 & 0.011 \\
  pan-left-right-4 &     28.563 &    858 &             858 & 322 & 0.375 &             858 &  86 & 0.100 &           759 & 254 & 0.335 \\
      randomized-1 &     39.730 &   1193 &            1193 & 401 & 0.336 &            1193 &  39 & 0.033 &           991 &   5 & 0.005 \\
      randomized-2 &     24.365 &    732 &             732 & 257 & 0.351 &             732 &  16 & 0.022 &           582 &  43 & 0.074 \\
      randomized-3 &     31.199 &    937 &             937 & 381 & 0.407 &             937 &  52 & 0.055 &           718 &  44 & 0.061 \\
      randomized-4 &     36.799 &   1105 &            1105 & 460 & 0.416 &            1105 & 168 & 0.152 &           814 & 162 & 0.199 \\
    tilt-up-down-1 &     29.998 &    901 &             901 &   0 & 0.000 &             901 &   0 & 0.000 &           793 &   0 & 0.000 \\
    tilt-up-down-2 &     41.301 &   1240 &            1240 &  53 & 0.043 &            1240 &  16 & 0.013 &          1083 &  11 & 0.010 \\
    tilt-up-down-3 &     29.632 &    890 &             890 &  40 & 0.045 &             890 &  21 & 0.024 &           779 &   0 & 0.000 \\
    tilt-up-down-4 &     37.931 &   1139 &            1139 & 367 & 0.322 &            1139 & 100 & 0.088 &          1000 & 267 & 0.267 \\
         up-down-1 &     33.167 &    996 &             996 &  50 & 0.050 &             996 &   3 & 0.003 &           874 &   0 & 0.000 \\
         up-down-2 &     31.998 &    961 &             961 & 223 & 0.232 &             961 &  10 & 0.010 &           845 &   0 & 0.000 \\
         up-down-3 &     39.030 &   1172 &            1172 & 132 & 0.113 &            1172 &   1 & 0.001 &          1039 &   0 & 0.000 \\
         up-down-4 &     33.298 &   1000 &            1000 & 247 & 0.247 &            1000 &  72 & 0.072 &           883 & 233 & 0.264 \\
\bottomrule
\end{tabular}

    \caption{The test cases for discontinuity rates of the bundle systems. $n$ is the number of detections, $d$ is the number of discontinuities, and $r_d=\frac{d}{n}$ is the discontinuity rate for each test case.}
    \label{table:bundle_discontinuity_test_cases}
\end{table}

\clearpage
\subsection{Speed Test Cases}
\label{appendix:speed_test_cases}

Tables~\ref{table:single_marker_speed_test_cases} and~\ref{table:bundle_speed_test_cases} outline the test cases for
the detection rates of the single marker and bundle systems respectively.
Test cases with the same base name but different indices (e.g.~z120cm-0 and z120cm-1) represent disjointed sections of
a longer, single video.

\begin{table}[h]
    \centering
    \begin{tabular}{|l|rrr|rrr|rrr|rrr|}
\toprule
Fiducial System & \multicolumn{3}{c|}{April Tag 24h10} & \multicolumn{3}{c|}{April Tag 48h12} & \multicolumn{3}{c|}{WhyCode Ellipse} & \multicolumn{3}{c|}{WhyCode Orig} \\
{} &      $\ell$ (s) &  $n$ & $F$ (Hz) &      $\ell$ (s) &  $n$ & $F$ (Hz) &      $\ell$ (s) &  $n$ & $F$ (Hz) &   $\ell$ (s) &  $n$ & $F$ (Hz) \\
Test Case           &                 &      &          &                 &      &          &                 &      &          &              &      &          \\
\midrule
z120cm-0            &            19.9 &  374 &     18.8 &            19.9 &  340 &     17.1 &            19.9 &  509 &     25.6 &         19.9 &  512 &     25.7 \\
z120cm-1            &            19.9 &  379 &     19.1 &            19.9 &  328 &     16.5 &            19.9 &  509 &     25.6 &         19.9 &  516 &     25.9 \\
z120cm-2            &            19.9 &  384 &     19.3 &            19.9 &  336 &     16.9 &            19.9 &  513 &     25.8 &         19.9 &  518 &     26.0 \\
z120cm-deflection-0 &            19.9 &  397 &     20.0 &            19.9 &  356 &     17.9 &            19.9 &  515 &     25.9 &         19.9 &  519 &     26.1 \\
z120cm-deflection-1 &            19.9 &  417 &     21.0 &            19.9 &  398 &     20.0 &            19.9 &  518 &     26.0 &         19.9 &  521 &     26.2 \\
z120cm-deflection-2 &            19.9 &  410 &     20.6 &            19.9 &  412 &     20.7 &            19.9 &  514 &     25.8 &         19.9 &  521 &     26.2 \\
z150cm-0            &            19.9 &  380 &     19.1 &            19.9 &  429 &     21.6 &            19.9 &  514 &     25.8 &         19.9 &  529 &     26.6 \\
z150cm-1            &            19.9 &  370 &     18.6 &            19.9 &  422 &     21.2 &            19.9 &  520 &     26.1 &         19.9 &  518 &     26.0 \\
z150cm-2            &            19.9 &  357 &     18.0 &            19.9 &  425 &     21.4 &            19.9 &  519 &     26.1 &         19.9 &  522 &     26.2 \\
z150cm-deflection-0 &            19.9 &  368 &     18.5 &            19.9 &  420 &     21.1 &            19.9 &  512 &     25.7 &         19.9 &  518 &     26.1 \\
z150cm-deflection-1 &            19.9 &  370 &     18.6 &            19.9 &  429 &     21.6 &            19.9 &  522 &     26.3 &         19.9 &  525 &     26.4 \\
z150cm-deflection-2 &            19.9 &  379 &     19.0 &            19.9 &  429 &     21.6 &            19.9 &  516 &     25.9 &         19.9 &  527 &     26.5 \\
z180cm-0            &            19.9 &  348 &     17.5 &            19.9 &  330 &     16.6 &            19.9 &  521 &     26.2 &         19.9 &  527 &     26.5 \\
z180cm-1            &            19.9 &  336 &     16.9 &            19.9 &  329 &     16.6 &            19.9 &  521 &     26.2 &         19.9 &  528 &     26.5 \\
z180cm-2            &            19.9 &  346 &     17.4 &            19.9 &  335 &     16.9 &            19.9 &  526 &     26.4 &         19.9 &  523 &     26.3 \\
z180cm-deflection-0 &            19.9 &  385 &     19.4 &            19.8 &  354 &     17.8 &            19.9 &  516 &     25.9 &         19.9 &  516 &     25.9 \\
z180cm-deflection-1 &            19.9 &  377 &     19.0 &            19.8 &  345 &     17.4 &            19.9 &  514 &     25.8 &         19.9 &  512 &     25.7 \\
z180cm-deflection-2 &            19.9 &  393 &     19.8 &            19.8 &  362 &     18.3 &            19.9 &  522 &     26.2 &         19.9 &  522 &     26.2 \\
z210cm-0            &            19.9 &  342 &     17.2 &            19.9 &  409 &     20.6 &            19.9 &  519 &     26.1 &         19.9 &  485 &     24.4 \\
z210cm-1            &            19.9 &  345 &     17.4 &            19.9 &  398 &     20.0 &            19.9 &  524 &     26.3 &         19.9 &  503 &     25.3 \\
z210cm-2            &            19.9 &  340 &     17.1 &            19.9 &  397 &     20.0 &            19.9 &  518 &     26.0 &         19.9 &  522 &     26.2 \\
z210cm-deflection-0 &            19.9 &  321 &     16.2 &            19.9 &  378 &     19.0 &            19.9 &  522 &     26.2 &         19.9 &  456 &     22.9 \\
z210cm-deflection-1 &            19.9 &  330 &     16.6 &            19.9 &  380 &     19.1 &            19.9 &  521 &     26.2 &         19.9 &  527 &     26.5 \\
z210cm-deflection-2 &            19.9 &  326 &     16.4 &            19.9 &  379 &     19.1 &            19.9 &  523 &     26.3 &         19.9 &  525 &     26.4 \\
z240cm-0            &            19.9 &  288 &     14.5 &            19.9 &  293 &     14.8 &            19.9 &  531 &     26.7 &         19.9 &  526 &     26.4 \\
z240cm-1            &            19.9 &  299 &     15.0 &            19.9 &  295 &     14.9 &            19.9 &  522 &     26.2 &         19.9 &  534 &     26.8 \\
z240cm-2            &            19.9 &  298 &     15.0 &            19.9 &  298 &     15.0 &            19.9 &  522 &     26.2 &         19.9 &  524 &     26.3 \\
z240cm-deflection-0 &            19.9 &  313 &     15.7 &            19.9 &  295 &     14.8 &            19.9 &  526 &     26.4 &         19.9 &  531 &     26.7 \\
z240cm-deflection-1 &            19.9 &  316 &     15.9 &            19.9 &  299 &     15.0 &            19.9 &  524 &     26.3 &         19.9 &  525 &     26.4 \\
z240cm-deflection-2 &            19.9 &  315 &     15.8 &            19.9 &  298 &     15.0 &            19.9 &  524 &     26.3 &         19.9 &  526 &     26.4 \\
z270cm-0            &            19.9 &  297 &     14.9 &            19.9 &  328 &     16.5 &            19.9 &  520 &     26.1 &         19.9 &  519 &     26.1 \\
z270cm-1            &            19.9 &  298 &     15.0 &            19.9 &  317 &     15.9 &            19.9 &  523 &     26.3 &         19.9 &  524 &     26.3 \\
z270cm-2            &            19.9 &  297 &     14.9 &            19.9 &  319 &     16.0 &            19.9 &  518 &     26.0 &         19.9 &  543 &     27.3 \\
z270cm-deflection-0 &            19.9 &  295 &     14.9 &            19.9 &  310 &     15.6 &            19.9 &  445 &     22.4 &         19.9 &  532 &     26.7 \\
z270cm-deflection-1 &            19.9 &  298 &     15.0 &            19.9 &  313 &     15.7 &            19.9 &  529 &     26.6 &         19.9 &  529 &     26.6 \\
z270cm-deflection-2 &            19.9 &  294 &     14.8 &            19.9 &  312 &     15.7 &            19.9 &  520 &     26.1 &         19.9 &  522 &     26.2 \\
z300cm-0            &            19.9 &  299 &     15.0 &            19.9 &  289 &     14.5 &            19.9 &  526 &     26.4 &         19.9 &  521 &     26.2 \\
z300cm-1            &            19.9 &  299 &     15.0 &            19.9 &  296 &     14.9 &            19.9 &  523 &     26.3 &         19.9 &  526 &     26.4 \\
z300cm-2            &            19.9 &  299 &     15.0 &            19.9 &  298 &     15.0 &            19.9 &  523 &     26.3 &         19.9 &  529 &     26.6 \\
z300cm-deflection-0 &            19.9 &  299 &     15.0 &            19.9 &  290 &     14.6 &            19.9 &  528 &     26.5 &         19.9 &  537 &     27.0 \\
z300cm-deflection-1 &            19.9 &  295 &     14.8 &            19.9 &  294 &     14.8 &            19.9 &  523 &     26.2 &         19.9 &  526 &     26.4 \\
z300cm-deflection-2 &            19.9 &  299 &     15.0 &            19.9 &  294 &     14.8 &            19.9 &  530 &     26.6 &         19.9 &  528 &     26.5 \\
\bottomrule
\end{tabular}

    \caption{The test cases for detection rates of the single marker systems. $\ell$ is the length in seconds of the test case, $n$ is the number of frames, $F$ is the detection rate in Hz.}
    \label{table:single_marker_speed_test_cases}
\end{table}

\begin{table}[h]
    \centering
    \begin{tabular}{|l|rrr|rrr|rrr|rrr|}
\toprule
Fiducial System & \multicolumn{3}{c|}{April Tag 24h10} & \multicolumn{3}{c|}{April Tag 48h12} & \multicolumn{3}{c|}{WhyCode Multi} \\
{} &      $\ell$ (s) &  $n$ & $F$ (Hz) &      $\ell$ (s) &  $n$ & $F$ (Hz) &    $\ell$ (s) &  $n$ & $F$ (Hz) \\
Test Case           &                 &      &          &                 &      &          &               &      &          \\
\midrule
z120cm-0            &            19.9 &  340 &     17.1 &            19.9 &  315 &     15.9 &          19.9 &  504 &     25.3 \\
z120cm-1            &            19.9 &  354 &     17.8 &            19.9 &  316 &     15.9 &          19.9 &  515 &     25.9 \\
z120cm-2            &            19.9 &  349 &     17.6 &            19.9 &  313 &     15.8 &          19.9 &  508 &     25.5 \\
z120cm-deflection-0 &            19.9 &  354 &     17.8 &            19.9 &  395 &     19.9 &          19.9 &  502 &     25.2 \\
z120cm-deflection-1 &            19.9 &  365 &     18.4 &            19.9 &  391 &     19.7 &          19.9 &  513 &     25.8 \\
z120cm-deflection-2 &            19.9 &  319 &     16.1 &            19.9 &  390 &     19.6 &          19.9 &  510 &     25.6 \\
z150cm-0            &            19.8 &  354 &     17.8 &            19.8 &  296 &     15.0 &          19.9 &  387 &     19.5 \\
z150cm-1            &            19.8 &  376 &     18.9 &            19.8 &  358 &     18.1 &          19.9 &  353 &     17.8 \\
z150cm-2            &            19.8 &  367 &     18.5 &            19.8 &  362 &     18.3 &          19.9 &  386 &     19.4 \\
z150cm-deflection-0 &            19.9 &  379 &     19.1 &            19.9 &  345 &     17.4 &          19.9 &  393 &     19.7 \\
z150cm-deflection-1 &            19.9 &  374 &     18.8 &            19.9 &  355 &     17.9 &          19.9 &  392 &     19.7 \\
z150cm-deflection-2 &            19.9 &  378 &     19.0 &            19.9 &  364 &     18.3 &          19.9 &  388 &     19.5 \\
z180cm-0            &            19.9 &  305 &     15.4 &            19.9 &  327 &     16.5 &          19.9 &  518 &     26.0 \\
z180cm-1            &            19.9 &  300 &     15.1 &            19.9 &  324 &     16.3 &          19.9 &  513 &     25.8 \\
z180cm-2            &            19.9 &  308 &     15.5 &            19.9 &  325 &     16.4 &          19.9 &  518 &     26.0 \\
z180cm-deflection-0 &            19.9 &  342 &     17.2 &            19.8 &  348 &     17.5 &          19.9 &  517 &     26.0 \\
z180cm-deflection-1 &            19.9 &  328 &     16.5 &            19.8 &  355 &     17.9 &          19.9 &  515 &     25.9 \\
z180cm-deflection-2 &            19.9 &  370 &     18.6 &            19.8 &  359 &     18.1 &          19.9 &  514 &     25.8 \\
z210cm-0            &            19.9 &  352 &     17.7 &            19.9 &  337 &     17.0 &          19.9 &  398 &     20.0 \\
z210cm-1            &            19.9 &  350 &     17.6 &            19.9 &  344 &     17.3 &          19.9 &  395 &     19.9 \\
z210cm-2            &            19.9 &  340 &     17.1 &            19.9 &  338 &     17.0 &          19.9 &  394 &     19.8 \\
z210cm-deflection-0 &            19.9 &  324 &     16.3 &            19.9 &  316 &     15.9 &          19.9 &  388 &     19.5 \\
z210cm-deflection-1 &            19.9 &  331 &     16.7 &            19.9 &  313 &     15.8 &          19.9 &  395 &     19.9 \\
z210cm-deflection-2 &            19.9 &  335 &     16.9 &            19.9 &  335 &     16.9 &          19.9 &  390 &     19.6 \\
z240cm-0            &            19.9 &  283 &     14.2 &            19.8 &  293 &     14.8 &          19.9 &  503 &     25.3 \\
z240cm-1            &            19.9 &  296 &     14.9 &            19.8 &  295 &     14.9 &          19.9 &  519 &     26.1 \\
z240cm-2            &            19.9 &  256 &     12.9 &            19.8 &  296 &     14.9 &          19.9 &  519 &     26.1 \\
z240cm-deflection-0 &            19.9 &  258 &     13.0 &            19.9 &  299 &     15.1 &          19.9 &  519 &     26.1 \\
z240cm-deflection-1 &            19.9 &  298 &     15.0 &            19.9 &  299 &     15.1 &          19.9 &  517 &     26.0 \\
z240cm-deflection-2 &            19.9 &  300 &     15.1 &            19.9 &  301 &     15.2 &          19.9 &  513 &     25.8 \\
z270cm-0            &            19.9 &  304 &     15.3 &            19.9 &  291 &     14.6 &          19.9 &  383 &     19.3 \\
z270cm-1            &            19.9 &  303 &     15.3 &            19.9 &  295 &     14.8 &          19.9 &  303 &     15.2 \\
z270cm-2            &            19.9 &  303 &     15.3 &            19.9 &  297 &     15.0 &          19.9 &  391 &     19.7 \\
z270cm-deflection-0 &            19.9 &  297 &     15.0 &            19.9 &  285 &     14.3 &          19.9 &  369 &     18.5 \\
z270cm-deflection-1 &            19.9 &  281 &     14.1 &            19.9 &  296 &     14.9 &          19.9 &  329 &     16.5 \\
z270cm-deflection-2 &            19.9 &  299 &     15.1 &            19.9 &  298 &     15.0 &          19.9 &  367 &     18.4 \\
z300cm-0            &            19.9 &  285 &     14.3 &            19.9 &  298 &     15.0 &          19.9 &  477 &     24.0 \\
z300cm-1            &            19.9 &  278 &     14.0 &            19.9 &  298 &     15.0 &          19.9 &  516 &     25.9 \\
z300cm-2            &            19.9 &  289 &     14.5 &            19.9 &  297 &     14.9 &          19.9 &  520 &     26.1 \\
z300cm-deflection-0 &            19.9 &  294 &     14.8 &            19.9 &  294 &     14.8 &          19.9 &  508 &     25.5 \\
z300cm-deflection-1 &            19.9 &  286 &     14.4 &            19.9 &  294 &     14.8 &          19.9 &  519 &     26.1 \\
z300cm-deflection-2 &            19.9 &  247 &     12.4 &            19.9 &  293 &     14.8 &          19.9 &  518 &     26.0 \\
\bottomrule
\end{tabular}

    \caption{The test cases for detection rates of the bundle marker systems. $\ell$ is the length in seconds of the test case, $n$ is the number of frames, $F$ is the detection rate in Hz.}
    \label{table:bundle_speed_test_cases}
\end{table}

\clearpage
\subsection{System Parameters}
\label{appendix:system_parameters}

The folllowing section shows the runtime parameters for the fiducial systems.
For the discontinuity tests, GUI and visualization functionalities (e.g.~\texttt{image\_view}) were enabled for debugging purposes for all systems.
These were disabled during the detection rate tests to reduce extraneous computational resource usage.
We show the system parameters for our tests in Tables~\ref{table:april_tag_parameters} and~\ref{table:whycode_parameters}.
Finally, we changed the tag definitions for the April Tag systems to include a bundle of all the tags during the bundle tests,
and to include only the largest of the tags during the single marker tests.

\begin{table}[h]
    \centering
    \begin{tabular}{lr}
    \toprule
        Parameter & Value(s) \\
    \midrule
        \texttt{tag\_family} & tagCustom24h10, tagCustom48h12 \\
        \texttt{tag\_threads} & 4 \\
        \texttt{tag\_decimate} & 1.0 \\
        \texttt{tag\_blur} & 0.0 \\
        \texttt{tag\_refine\_edges} & 1 \\
        \texttt{tag\_debug} & 0 \\
        \texttt{max\_hamming\_dist} & 1 \\
        \texttt{publish\_tf} & false \\
    \bottomrule
    \end{tabular}
    \caption{The April Tag system parameters. We have changed the tag family based on which family was tested.}
    \label{table:april_tag_parameters}
\end{table}

\begin{table}[h]
    \centering
    \begin{tabular}{lr}
    \toprule
        Parameter & Value(s) \\
    \midrule
        \texttt{identify} & true \\
        \texttt{circleDiameter} & 0.123, 0.3 \\
        \texttt{numMarkers} & 4,3 \\
        \texttt{minSize} & 30 \\
        \texttt{fieldLength} & 1.0 \\
        \texttt{fieldWidth} & 1.0 \\
        \texttt{initialCircularityTolerance} & 100.0 \\
        \texttt{finalCircularityTolerance} & 2.0 \\
        \texttt{areaRatioTolerance} & 40.0 \\
        \texttt{centerDistanceToleranceRatio} & 10.0 \\
        \texttt{centerDistanceToleranceRatioAbs} & 5.0 \\
        \texttt{id\_bits} & 8 \\
        \texttt{id\_samples} & 360 \\
        \texttt{pub\_visual} & true, false \\
        \texttt{pub\_tf} & true, false \\
        \texttt{use\_gui} & true, false \\
    \bottomrule
    \end{tabular}
    \caption{The WhyCode system parameters. A \texttt{circleDiameter} of 0.123 corresponds to the markers in the WhyCode Multi marker, and 0.3 corresponds to the others.
    When testing for discontinuities (on a desktop) \texttt{pub\_visual}, \texttt{pub\_tf}, and \texttt{use\_gui} were set to true for visualization purposes.
    When testing for detection rate on the Raspberry Pi (in headless mode), all of these were set to false to save on computational resources.}
    \label{table:whycode_parameters}
\end{table}

%\subsection{All Figures}
%\input{autogenerated/auto_generated_appendix_figures.tex}
%
%\newpage
%\subsection{Aggregated Data}
%\input{autogenerated/auto_generated_table_all.tex}
